# Supplementary material for: Evidence for a correlated insulator to antiferromagnetic metal transition in CrN
Source: arXiv:1004.0042 source file (2010-04-01)
Supplement: Supplementary file 1 [file CrN_res_supplementary01.pdf]

*Supplementary Material to the paper titled:*

# Evidence for a correlated insulator to antiferromagnetic metal transition in CrN

## Resistivity Analysis of CrN

Chromium Nitride used in the present experiment was characterized for its magnetic and electrical transport properties and found to be consistent with reports indicating a first order magneto-structural transition in CrN[1]. The antiferromagnetic ordering temperature, as determined from the magnetic susceptibility measurements, was found to be $T_N \sim 286$ K. A sharp step-like feature is observed in the region around $T_N$ with hysteresis of $\sim 4$ K in warming and cooling data sets of resistivity(inset to Fig. 1). This is a signature of the first order nature of the antiferromagnetic transition. The electrical resistivity above $T_N$ shows an activation energy of 70 meV (as discussed in the paper) and confirms the insulating state above $T_N$. While the resistivity below $T_N$ also exhibits a negative temperature coefficient of resistivity, it does not follow an activated behavior(Fig. 1). Rather, a $ln\rho$ versus $1/T$ yields a very small value of slope indicative of a gap (if any) in sub-meV range. Also we estimate the maximum resisitivity, $\rho_0 \sim 0.022$ Ω-cm for T→ 0 in the present case, while that inferred from the recent data of C. X. Quintela *et.al* [1] is about 100 Ω-cm.

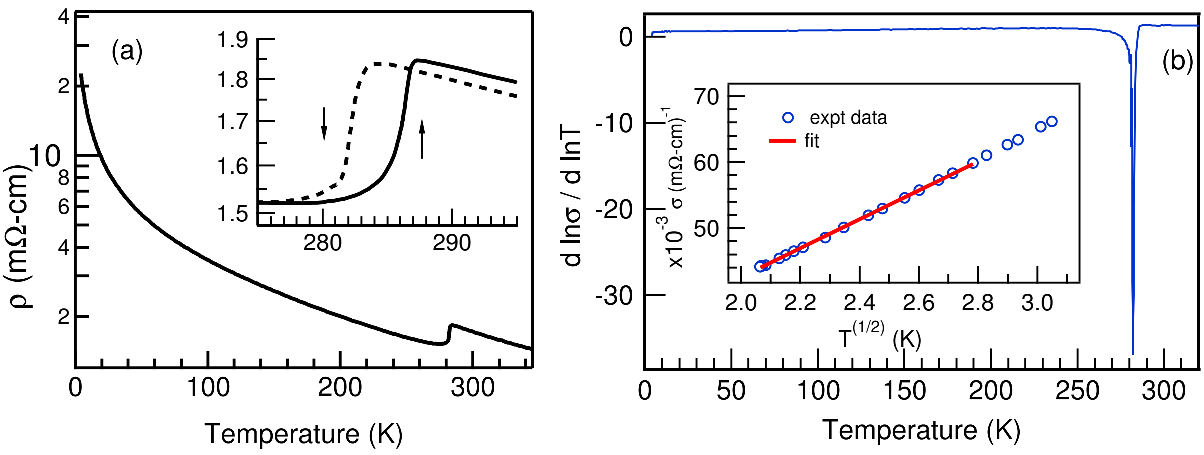


FIG. 1: (Colour online)(a) The temperature dependence of resistivity with inset showing the signature of first order antiferromagnetic transition. (b) The plot of d($ln\sigma$)/d($lnT$) vs T extrapolates to zero with $T \rightarrow 0$ typical of a metallic system. A fit to the data using equation $\sigma(T) = \sigma(0) + mT^{1/2}$ indicative of a correlated metal in the presence of disorder is shown in the inset.

To investigate the low temperature electronic transport behaviour of CrN, we thus applied the Möbius criterion [2] to the resistivity data. As per this criterion, the derivative d($ln\sigma$)/d($lnT$) for a metal extrapolates to zero with $T \rightarrow 0$ as the conductivity, $\sigma$, is a finite value at $T \rightarrow 0$ for metallic systems. In contrast, d($ln\sigma$)/d($lnT$) would diverge as $T \rightarrow 0$ for systems with $\sigma$ that follow an exponential dependence on $T$. In the present case, the d($ln\sigma$)/d($lnT$) versus $T$ tends to zero as indicated in Fig. 1. In fact, the conductivity can be fitted to a $T^{1/2}$, typical of a correlated metal in the presence of disorder [3, 4], as is also known for metallic heavily doped Si, $La_{2-x}Sr_xCuO_4$, $LaNi_{1-x}Co_xO_3$, etc [2, 5, 6]. We do confirm the presence of strong electron electron correlations of the order of 4.5 eV in CrN through resonant photoelectron spectroscopy as presented in the main paper.

The overlap of the defect impurity band with the conduction band can lead to a degenerate Fermi-gas limit. The origin of disorder or impurity defect in CrN is generally the off-stoichiometry of Nitrogen. For example, the effect of variation of $x$ in $CrN_x$ was studied in polycrystalline samples by Browne *et.al.*(Ref. [7]). The sample with a highly stoichiometric N composition of $x = 0.997$ displayed a sharp first order antiferromagnetic transition at $T_N = 286$ K. It also displayed a hysteresis of 2 - 3 K as measured by linear expansivity, susceptibility, and resistivity. While the transition in a sample with $x = 0.98$ was found to be broad and occured at $T_N = 273$ K. Furthermore, thin films of polycrystalline $CrN_x$ with $1.0 \leq x \leq 1.2$ studied by Tsuchiya *et al.*[8] also showed behavior similar to the samples of Browne *et al.*. Thus, the Nitrogen stoichiometry in CrN is known to greatly influence its properties. Keeping CrN defect free in this aspect had been quite difficult in the past. However, the N 1$s$ core-level spectrum presented at Fig . 2 confirms the stiochiometry of the CrN sample used in the present study.

Firstly, no additional feature is observed at higher binding energy to the main peak which confirms high quality of the sample surface. Further, the binding energy for the N 1$s$ peak is 396.6 ± 0.1 eV. It was shown [9] that the binding energy is characteristic of the stoichiometry and a highly stoichiometric sample showed a binding energy of 396.5 ± 0.1 eV. While, the samples with N deficiency ($CrN_{0.82}$) showed a clear deviation to 397 ± 0.1e V [9]. The position of N 1$s$ for the present sample also shows good agreement with the more recent report by F. Rivadulla et.al [10].

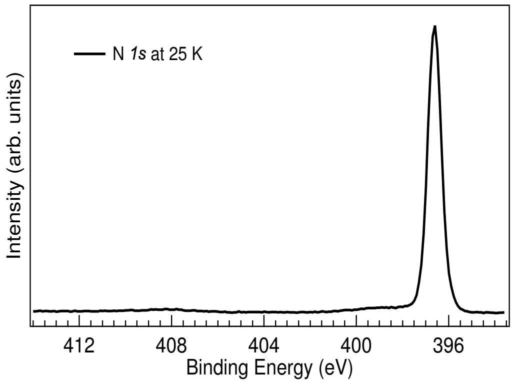


FIG. 2: A clean N 1$s$ core-level spectrum in CrN indicating high quality of the sample.

**Experimental details: Photoelectron Spectroscopy**

The soft x-ray Photoelectron Spectroscopy (PES) experiments were performed using synchrotron radiation at beamline BL17SU, SPring-8. XAS was recorded in the total electron yield mode. PES was obtained using a hemispherical electron analyzer, Gammadata-Scienta SES2002 with the total energy resolution set to 200 meV. These spectra were normalized to scan time and incident photon flux. Laser PES was performed using a Scienta R4000WAL electron analyzer and a vacuum-ultraviolet laser (h$\mu$= 6.994 eV) [11]. The total energy resolution was set to 6 meV at 5 K. Hard X-ray PES of the $Cr2p$ core-levels were measured at beamline BL29XU, SPring-8. A vacuum below 4 x $10^{-8}$ Pa was maintained throughout the measurements. Clean sample surfaces were obtained by cleaving *in situ* at low temperature. All the spectra were calibrated using the Fermi level measured from a gold film evaporated onto the sample holder. The measurements were carried out above (at 300 K) and below (at 25 K) the magneto-structural transition, in order to compare the spectra for the two phases. The Hard X-ray core level PES measurements were also carried out at 250 K. Temperature dependent measurements were carried out using a liquid He flow-type cryostat and were checked for reproducibility on T-cycling.

**Deatils of Cr 2$p$ core-level Cluster Model calculations**

We evidence a T-dependent “satellite” feature (575 eV) to the “main peak” feature (575.9 eV) in the bulk sensitive Hard X-ray Cr 2$p$ core-level PES as presented in Fig. 3 of the paper. A significant change in intensity occurs between the T = 300 K and 250 K spectra and then

the spectrum did not change down to 20 K, thus indicative of changes only across $T_N$. Similar well-screened features at the lower BE side of the main peak in core-level PES has been reported in several transition metal oxides with a direct relation to a metal-insulator transition, either as a function of T or doping [13, 14].

To account for such *extra* features within the framework of cluster model calculations, we introduced a charge transfer from a coherent band at $E_F$ in addition to the usual configuration of states in the $CrN_6$ cluster. The ground state is described by a linear combination of $3d^3$, $3d^4\underline{L}$, $3d^5\underline{L}^2$, $3d^4\underline{C}$, $3d^5\underline{LC}$ and $3d^5\underline{C}^2$, where $C$ and $L$ represent a hole in the coherent state and a hole in N $2p$ ligand state, respectively. As shown originally in Ref. [12], such a charge transfer from the coherent states can be directly related to the metallic screening in the core-level PES. In other words, we introduce the state $C$ at $E_F$ and define the parameters: $\Delta^*$ - the charge transfer energy between Cr $3d$ and $C$ and ${V_{eq}}^*$ - the hybridization between Cr $3d$ and $C$. These parameters are analogous to those associated with the Nitrogen ligand states *viz.* charge transfer energy $\Delta$ between Cr $3d$ and N $2p$ states, and hybridization $V_{eq}$ between Cr $3d$ and N $2p$ states. We allow the $3d$-band hybridization to be reduced by a factor $R_c$ = 0.8d in the presence of the core hole and enhanced by the factor $1/R_v = 1/0.9$ in the presence of an extra $3d$ electron.

The other parameters were fixed to $U_{dd}$ = 4.5 eV obtained from the resonant PES experiment, charge transfer energy $\Delta$ = 2.5 eV, the crystal field splitting 10Dq = 1.5 eV, Coulomb interaction between Cr $3d$ and Cr $2p$ core hole states $U_{dc}$ = 6.5 eV and hybridization between Cr $3d$ and N $2p$ states $V_{eq}$ = 2.7 eV for all the temperatures. ${V_{eq}}^*$ and $\Delta^*$ were refined to obtain the fit with experimental spectra and best fit was attained for:

- ${V_{eq}}^* = 0.675$ eV and $\Delta^* = 0.4$ eV at 300 K
- ${V_{eq}}^* = 0.729$ eV and $\Delta^* = 0.6$ eV at 250 K
- ${V_{eq}}^* = 0.756$ eV and $\Delta^* = 0.7$ eV at 20 K

Thus calculated spectra showed good agreement with the experimental data. Morevoer, the inclusion of the screening channel is justified for the 300 K spectrum as the thermal broadening at $E_F(4K_BT \sim 100$ meV) is larger than the gap of 70 meV, known from the resisitivity measurments. Thus the thermal broadening reflects in the spectroscopic mea-

surements by overcoming the gap of 70 meV.

---


[1] C. X. Quintela, F. Rivadulla, and J. Rivas, Appl. Phys. Lett. **94**, 152103 (2009).

[2] A. Möbius, Solid. State. Commun. **73**, 215 (1990).

[3] P. A. Lee and T. V. Ramakrishnan, Rev. Mod. Phys. **57**, 287 (1985).

[4] T. F. Rosenbaum, K. Andres, G. A. Thomas, and P.A. Lee, Phys. Rev. Lett. **46**, 568 (1981).

[5] T. F. Rosenbaum and S. A. Carter, J. Solid. State. Chem. **88**, 94 (1990).

[6] K. P. Rajeev, G. V. Shivshankar, and A. K. Raychaudhuri, Solid. State. Commun. **79**, 591 (1991); K. P. Rajeev and A. K. Raychaudhuri, Phys. Rev. B **46**, 1309 (1992).

[7] J. D. Browne, R. R. Liddell, R. Street, and T. Mills, Phys. Status Solidi **1**, 715 (1970).

[8] Y. Tsuchiya, K. Kosuge, S. Yamaguchi, and N. Nakayama, Mater. Trans. JIM **37**, 121 (1996).

[9] I. Bertóti, M. Mohai, P. H. Mayrhofer, C. Mitterer, Surf. Interface Anal. **34**, 740 (2002).

[10] Francisco Rivadulla , Manuel Bañobre-López, Camilo X. Quintela, Alberto Piñeiro, Victor Pardo, Daniel Baldomir, Manuel Arturo López-Quintela, José Rivas, Carlos A. Ramos, Horacio Salva, Jian-Shi Zhou and John B. Goodenough, Nature Mater. **8**, 947 (2009).

[11] T. Kiss, F. Kanetaka, T. Yokoya, T. Shimojima, K. Kanai, S. Shin, Y. Onuki, T. Togashi, C. Zhang, C. T. Chen, and S. Watanabe, Phys. Rev. Lett. **94**, 057001 (2005).

[12] A. Kotani and Y. Toyozawa, J. Phys. Soc. Jpn. **37**, 912 (1974).

[13] M. Taguchi, A. Chainani, N. Kamakura, K. Horiba, Y. Takata, M. Yabashi, K. Tamasaku, Y. Nishino, D. Miwa, T. Ishikawa, S. Shin, E. Ikenaga, T. Yokoya, K. Kobayashi, T. Mochiku, K. Hirata, and K. Motoya, Phys. Rev. B **71**, 155102 (2005).

[14] K. Horiba, M. Taguchi, A. Chainani, Y. Takata, E. Ikenaga, D. Miwa, Y. Nishino, K. Tamasaku, M. Awaji, A. Takeuchi, M. Yabashi, H. Namatame, M. Taniguchi, H. Kumigashira, M. Oshima, M. Lippmaa, M. Kawasaki, H. Koinuma, K. Kobayashi, T. Ishikawa, and S. Shin, Phys. Rev. Lett. **93**, 236401 (2004).
